# Supplementary material for: From concrete mixture to structural design -- a holistic optimization procedure in the presence of uncertainties
Source: arXiv:2312.03607 source file (2023-12-06)
Supplement: Supplementary file 1 [file appendix_1.tex]

An appendix contains supplementary information that is not an essential part of the text itself but which may be helpful in providing a more comprehensive understanding of the research problem or it is information that is too cumbersome to be included in the body of the paper.

%%=============================================%%
%% For submissions to Nature Portfolio Journals %%
%% please use the heading ``Extended Data''.   %%
%%=============================================%%
